# Supplementary material for: SURF: Signature-Retained Fast Video Generation
Source: arXiv:2603.21002 source file (2026-05-18)
Supplement: Supplementary file 1 [file supp.tex]

\appendix
\section*{Supplementary}
\tableofcontents
% \newpage
\section{Project Page}
Our project page is included in the supplementary.zip.  
Please open \textbf{\texttt{SURF\_project\_website/index.html}} to view all demonstration videos.
Due to the overall upload size limit, all comparison videos are compressed with the same extent.
\section{Implementation Details}
\subsection{Base Models Configuration}
\label{sup:base_model}
In this section, we describe the configures of our baseline models. We adopt the original model implementations whenever possible.

\noindent \textbf{Wan2.1}~\citep{wan2025}: A 14-billion-parameter open-source video generation model. Wan2.1 ranks high in Physical Plausibility, ID Consistency, Scene Generation Quality etc. 
However with high-parameter and quadratic attention calculations for high-resolution (720p or 1080p), it suffers from large computation consume. 
It roughly uses over 50min to generate one 81frame 720p video on A800 80G with FA2~\citep{dao2023flashattention}. 

\noindent \textbf{HunyuanVideo}~\citep{kong2024hunyuanvideo}: A 13-billion-parameter open-source video generation model. HunyuanVideo is recognized for its smooth motion synthesis, precise semantic alignment, and high-quality aesthetics
It roughly uses over 50min to generate one 129frame 720p video on A800 80G with FA2~\citep{dao2023flashattention}. 

\noindent \textbf{AccVideo}~\citep{zhang2025accvideo}: Built upon HunyuanVideo, AccVideo introduces an efficient distillation-based acceleration framework that leverages synthetic datasets to significantly speed up video diffusion models.
This method is adaptable to both Wan2.1 and HunyuanVideo models. In this work, we utilize the model based on HunyuanT2V. It takes approximately 6 minutes to generate a 129-frame, 720p video on an A800 80G GPU using FA2\citep{dao2023flashattention}.

\noindent \textbf{Refiner}: We use an internal 1-billion-parameter transformer-based latent diffusion model ~\citep{peebles2023scalable} as the base T2V generation model, as illustrated in Fig.~\ref{fig:dit_backbone}. 
We employ a 3D-VAE to transform videos from the pixel space to a latent space, upon which we construct a transformer-based video diffusion model. Unlike previous models that rely on UNets or transformers, which typically incorporate an additional 1D temporal attention module for video generation, such spatially-temporally separated designs do not yield optimal results. 
We replace the 1D temporal attention with 3D self-attention, enabling the model to effectively perceive and process spatiotemporal tokens, thereby achieving a high-quality and coherent video generation model. 
Specifically, before each attention or feed-forward network (FFN) module, we map the timestep to a scale, thereby applying RMSNorm to the spatiotemporal tokens.
It is worth noting that the origin model does not support video generation at 720p resolution. 

\begin{figure*}[ht]
\centering
\includegraphics[width=1\linewidth]{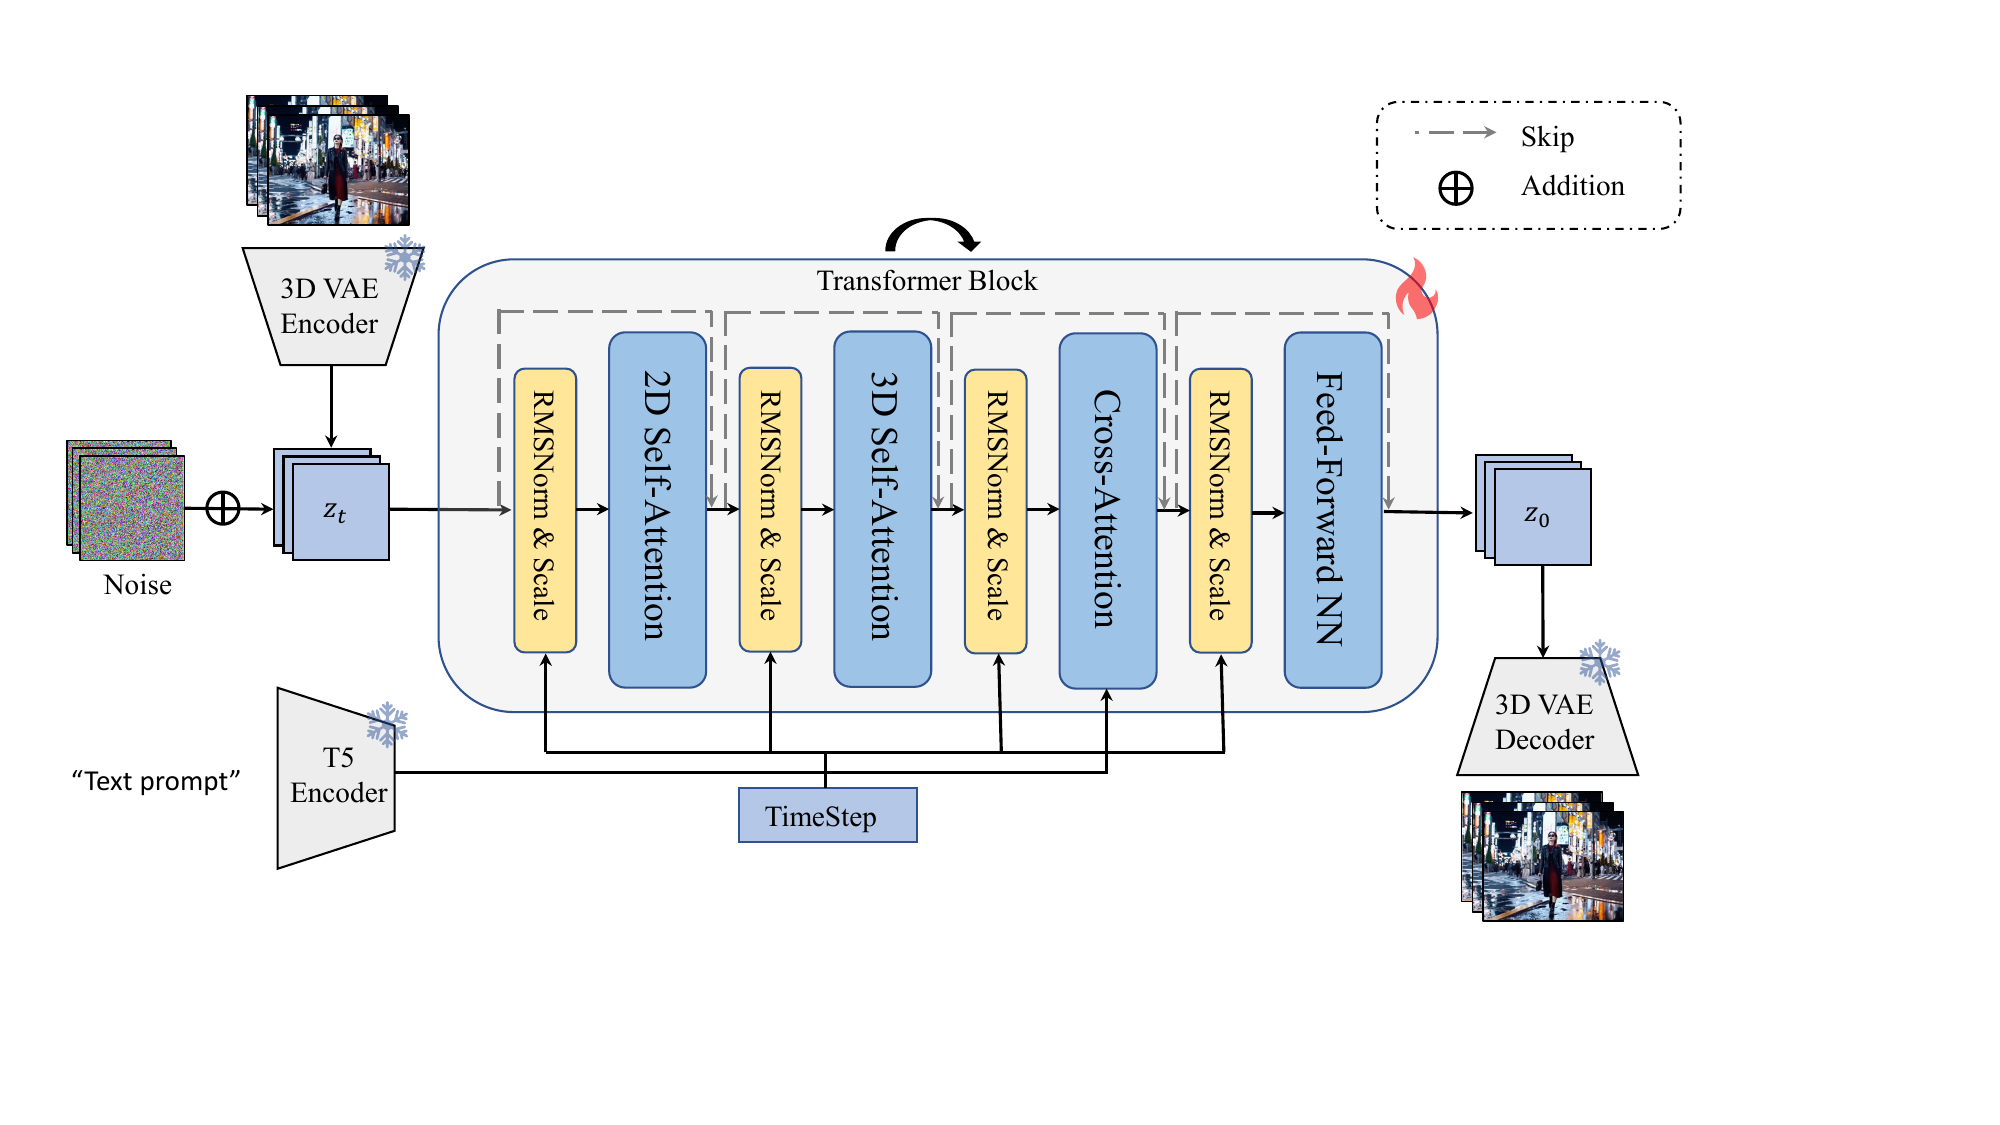}
\caption{\textbf{Overview of the base text-to-video generation model.} }
\label{fig:dit_backbone}
\end{figure*}
\subsection{Training Details}
\label{supp:traindetail}

We train the Refiner to transform a blurred video into a clear one while simultaneously refining unreasonable details. 
Specifically, we adopt flow matching~\citep{esser2024scaling} to map the low-resolution latent representation $Z_{LR}$ to the high-resolution latent representation $Z_{HR}$.  
Intermediate points are obtained via linear interpolation between $Z_{LR}$ and $Z_{HR}$. The training loss is defined with the target $Z_{LR} - Z_{HR}$. We randomly sample $t \sim \text{LogitNorm}[0,1]$ with a timestep shift of $5$, and compute: 
\[
Z_{t} = (1 - t) \cdot Z_{HR} + t \cdot Z_{LR}.
\]  
Using the $t$-independent target $Z_{LR} - Z_{HR}$ results in a straighter ODE trajectory, thereby enabling few-step generation.  
Since we divide \method into a preview stage and a refine stage, we also provide the corresponding configurations for different stages, as summarized in Tab.~\ref{tab:stage_config}.  

\begin{table}[t]
\centering
\caption{Configurations for different stages. 
A dash ($-$) indicates that the stage is \textit{training-free}.}
\label{tab:stage_config}
\small
\setlength{\tabcolsep}{1.5pt} % reduce column spacing
\begin{tabular}{cccc}
\toprule
\multirow{2}{*}{\textbf{Configuration}} & \multicolumn{2}{c}{\textbf{Preview Stage}} & \multirow{2}{*}{\textbf{Refine Stage}} \\
\cmidrule(lr){2-3}
& Pre-$k$ Steps & Post-$k$ Steps & \\
\midrule
Model Params & 14B & 14B & 1B \\
Dimension & 5120 & 5120 & 1152 \\
num\_heads & 40 & 40 & 16 \\
Optimizer & - & - & AdamW \\
Learning rate & - & - & $5\times10^{-5}$ \\
Numerical precision & bfloat16 & bfloat16 & bfloat16 \\
Resolution & 480p & 240p & 720p \\
timestep\_shift & 3 & 3 & 1 \\
CFG & 7.5 & 5 & 6 \\
\bottomrule
\end{tabular}
\end{table}

\subsection{Dataset Construction} 
\label{sec:dataset}
We collect approximately 100K high-quality video clips from the Internet to construct our training dataset. 
Given the highly variable quality of online videos, we follow the automated filtering pipeline proposed in \citep{xie2025simplegvr} to retain visually high-quality content. 

Specifically, we first discard videos that are overly bright or overly dark. 
For each remaining video, we uniformly sample 10 frames and compute two metrics: the average MUSIQ score~\citep{ke2021musiq} and the Laplacian variance, which reflects the level of spatial detail and sharpness. 
Videos with an average MUSIQ score below 40 or a Laplacian variance below 30 are discarded. 

To simulate degradations, we apply both pixel-level and latent-level operations. 
At the pixel level, we follow \citep{wang2021realesrgan} to synthesize corresponding LR–HR video pairs. 
At the latent level, we inject noise sampled from the range $[0.6, 0.9]$. 

We train \method on resolutions 720p and 1080p, while fixing the target FPS to 16 via frame skipping. 
For this multi-resolution training, we adopt aspect-ratio bucketing with a minimum unit size of 32 pixels. 
Since \method focuses on dynamically selecting suitable resolutions, frequent scale changes occur during inference and training. 
For clarity, we list the resolution buckets in Tab.~\ref{tab:resolution_settings}. 
\begin{table}[t]
\centering
\caption{\textbf{Resolution settings across different aspect ratios.} 
We report the spatial dimensions (height, width) for 1080p, 720p, 480p, and 240p under square ($1{:}1$) and portrait ($9{:}16$) aspect ratios.}
\small
\setlength{\tabcolsep}{2.5pt}
\begin{tabular}{c|c|c|c|c}
\toprule
\textbf{Aspect Ratio} & \textbf{1080p} & \textbf{720p} & \textbf{480} & \textbf{240p} \\
\midrule
$1{:}1$   & (1440, 1440) & (960, 960)   & (576, 576)   & (336, 336) \\
$9{:}16$  & (1080, 1920) & (720, 1280)  & (480, 832)   & (240, 416) \\
\bottomrule
\end{tabular}
\label{tab:resolution_settings}
\end{table}

\subsection{Evaluation Metrics}

For text-to-video evaluation, we randomly select 381 prompts, consisting of 326 prompts from the benchmark VBench~\citep{huang2024vbench}, 20 prompts from Videophy~\citep{bansal2024videophy}, and 35 prompts from PhyGenBench~\citep{meng2024towards}. 
Our evaluation protocol measures video quality from both global and local perspectives. 
To this end, we employ a comprehensive suite of automated metrics: 
\textit{Quality Score (QS), Aesthetic Quality (AQ), Dynamic Degree (DD), Motion Smoothness (MS), Overall Consistency (OC)} for general video evaluation, and 
\textit{Semantic Adherence (SA)} and \textit{Physics Commonsense (PC)} for physical plausibility.  

\noindent\textbf{Quality Score (QS).}  
The weighted average of multiple dimensions, including subject consistency, background consistency, temporal flickering, motion smoothness, aesthetic quality, imaging quality, and dynamic degree.  

\noindent\textbf{Aesthetic Quality (AQ).}  
Assesses the artistic and aesthetic value of each frame using the LAION aesthetic predictor~\citep{schuhmann2022laion}. It reflects high-level properties such as composition, color harmony, and photorealism.  

\noindent\textbf{Dynamic Degree (DD).}  
Quantifies the magnitude of motion using optical flow fields estimated by RAFT~\citep{teed2020raft}. This metric discourages static or near-static generations and promotes natural motion in dynamic scenes.  

\noindent\textbf{Motion Smoothness (MS).}  
Measures the temporal smoothness of motion using a video frame interpolation model~\citep{li2023amt}.  

\noindent\textbf{Overall Consistency (OC).}  
Computed by ViCLIP~\citep{wang2023internvid} on general text prompts, reflecting both semantic and stylistic consistency.  

\noindent\textbf{Semantic Adherence (SA).}  
Measures the alignment between the generated video and the input text prompt~\citep{bansal2024videophy}. SA = 1 indicates that the caption is well grounded in the generated video.  

\noindent\textbf{Physics Commonsense (PC).}  
Assesses whether the generated video intuitively follows real-world physical laws. PC = 1 indicates that object dynamics, interactions, and motions align with human commonsense physics.  
For evaluation, we consider PC and SA return values greater than or equal to 0.5 as PC = 1 and SA = 1, and values less than 0.5 as PC = 0 and SA = 0.

\vspace{0.5em}
\noindent\textbf{Evaluation of 1080p Videos.}  
We further evaluate 1080p videos from the perspective of super-resolution quality. Specifically, we calculate the DINO~\citep{caron2021emerging} feature similarity across frames, evaluate the temporal consistency of the background scenes by
calculating CLIP~\citep{radford2021learning} feature similarity across frames, use the LAION aesthetic predictor~\citep{schuhmann2022laion} to measure aesthetic quality, and DOVER~\citep{wu2023exploring} to assess overall video quality.  

\subsection{Details of User Study}
Fig.~\ref{fig:user_study_form} shows the Google Form questionnaire used in our user study to present video assets. We randomly sampled 24 prompts and constructed different comparison pairs with randomized orders to avoid positional bias.
To ensure data reliability, we filtered out invalid responses in which participants consistently selected the same option across all four questions (e.g., always choosing "left video" or "same").
After this filtering, a total of 37 valid questionnaires remained, and the corresponding results are reported in Experiment.

\begin{figure}[t]
    \centering 
    \includegraphics[width=0.98\linewidth]{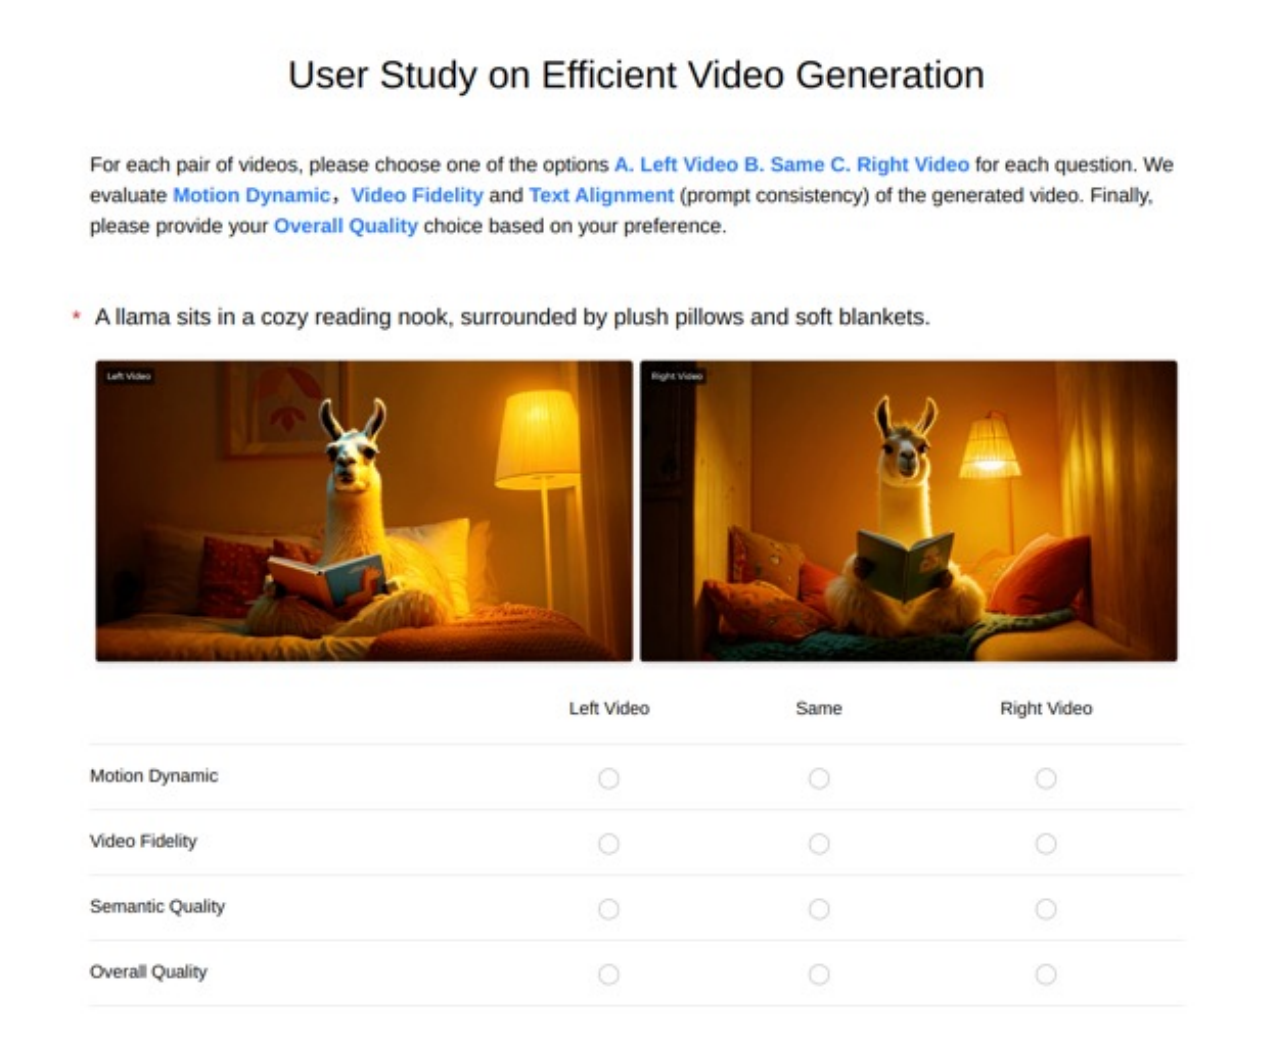} 
    \caption{%
            \textbf{User study} questionnaire form example.
    }
    \label{fig:user_study_form}
    \vspace{-10pt}
\end{figure}

\section{Additional Experimental Results}
\subsection{Comparisons}

In this section, we first compare the preview (240p) generated by \method with the same resolution generated by Wan2.1.  
We conducted the user study using a standard win-rate methodology.  
We randomly selected 30 pairs of videos between \method's preview and Wan2.1.  
Participants indicated their preferences across three key dimensions: Motion Dynamics, Text Alignment, and Overall Quality.  
A total of 60 completed feedback forms were collected.  
We report the percentage of each option.
The results presented in Tab.~\ref{tab:userstudy_preview} demonstrate that our method is significantly preferred over the competing method.  
This outcome aligns with our experimental design, confirming that OptimRes-LowRes flow preserves superior spatial layout and maintains greater semantic alignment.

\begin{table}[t]
    \centering
    \caption{
        \textbf{User preference comparison} between \method's preview and Wan2.1 240p.
    }
    \label{tab:userstudy_preview}
    \small
    \setlength{\tabcolsep}{10pt}
    \begin{tabular}{lccc}
        \toprule
        \textbf{Metrics}& \textbf{Better} & \textbf{Same} & \textbf{Worse} \\
        \midrule
        Motion Dynamics  & 76.17 & 19.50 & 4.33 \\
        Text Alignment   & 83.37 & 13.96 & 2.67 \\
        Overall Quality  & 82.50 & 8.28  & 9.22 \\
        \bottomrule
    \end{tabular}
\end{table}

\begin{table}[t]
    \centering
    \caption{
        \textbf{User preference comparison} between \method and FlashVideo.
    }
    \label{tab:userstudy_flashvideo}
    \small
    \setlength{\tabcolsep}{10pt}
    \begin{tabular}{lccc}
        \toprule
        \textbf{Metrics} & \textbf{Better} & \textbf{Same} & \textbf{Worse} \\
        \midrule
        Motion Dynamics & 67.72 & 24.91 & 7.37 \\
        Video Fidelity  & 80.43 & 16.02 & 3.55 \\
        Text Alignment  & 69.03 & 24.35 & 6.61 \\
        Overall Quality & 89.24 & 5.27  & 5.49 \\
        \bottomrule
    \end{tabular}
\end{table}

\begin{figure*}[t]
\centering 
\includegraphics[width=0.98\linewidth]{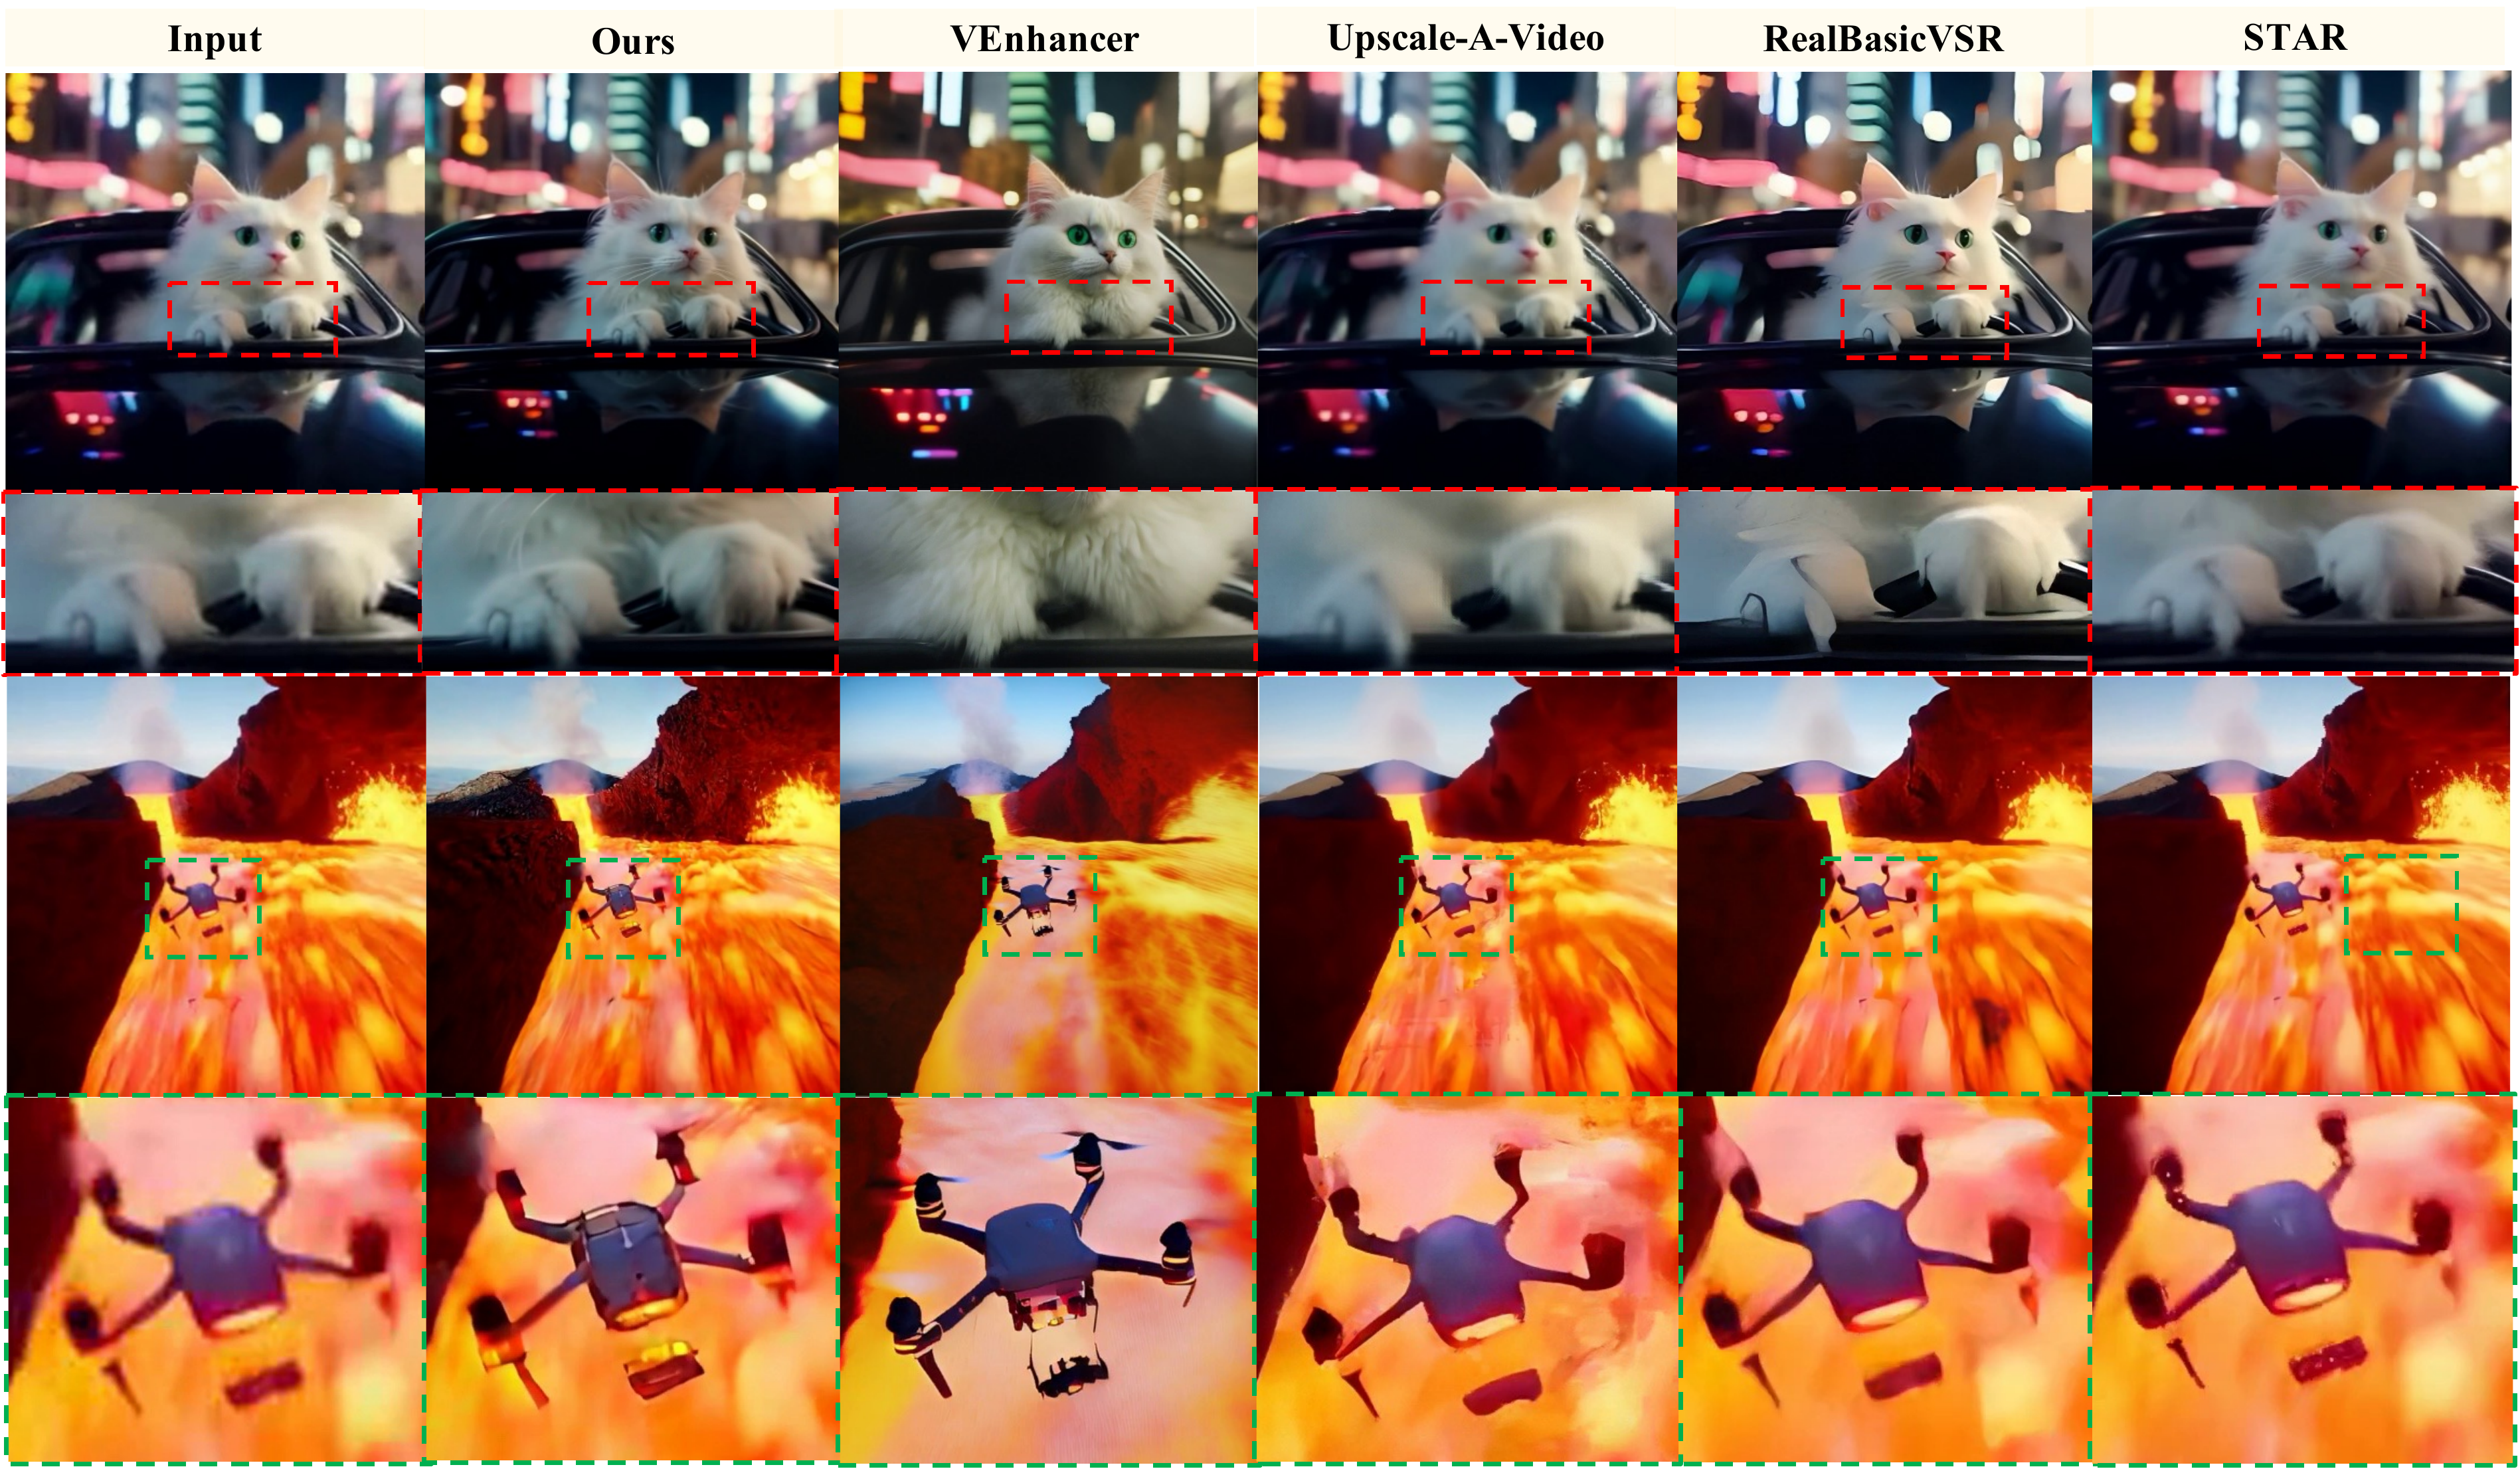} 
\vspace{-10pt}
\caption{%
    \textbf{Comparison with Various Video Enhancement Methods.}  
    Our method achieves more perceptually realistic and detail-rich refinement based on the initial low-resolution previews, outperforming other approaches in consistency and visual fidelity. Specific observations for each row are annotated beneath the corresponding frames.
}
\label{fig:CompareVSRframe}
\vspace{-10pt}
\end{figure*}

We also compare \method with cascaded video generation, using FlashVideo~\citep{zhang2025flashvideo} as an example.  
As shown in Fig.~\ref{fig:CompareVSRflashvideo}, our method generates more complex motions, achieves better text alignment, and offers enhanced visual refinement, resulting in higher overall visual quality.  
Quantitative results are shown in Tab.~\ref{tab:compareflash}.

\begin{table}[t]
    \centering
    \small
    \caption{\textbf{Comparison} between \method and FlashVideo. Highest value in \textbf{bold}.}
    \setlength{\tabcolsep}{8pt}
    
    \begin{tabular}{lccccc}
    \toprule
    \textbf{Method} & \textbf{QS $\uparrow$} & \textbf{AQ $\uparrow$} & \textbf{DD $\uparrow$} & \textbf{MS $\uparrow$} & \textbf{OC $\uparrow$} \\
    \midrule
    Flashvideo & 82.99 & 62.55 & 63.47 & 96.84 & \textbf{27.65} \\
    \method & \textbf{83.24} & \textbf{66.86} & \textbf{72.22} & \textbf{97.95} & 27.38  \\
    \bottomrule
    \end{tabular}
    \label{tab:compareflash}
\end{table}

Additionally, we conducted a user study with expanded evaluation criteria.  
We introduced "Video Fidelity" dimension, specifically focusing on visual noise and artifacts in the generated videos.  
As shown in Tab.~\ref{tab:userstudy_flashvideo}, \method outperforms FlashVideo in terms of user preference.

\begin{figure}[t]
\centering 
\includegraphics[width=0.98\linewidth]{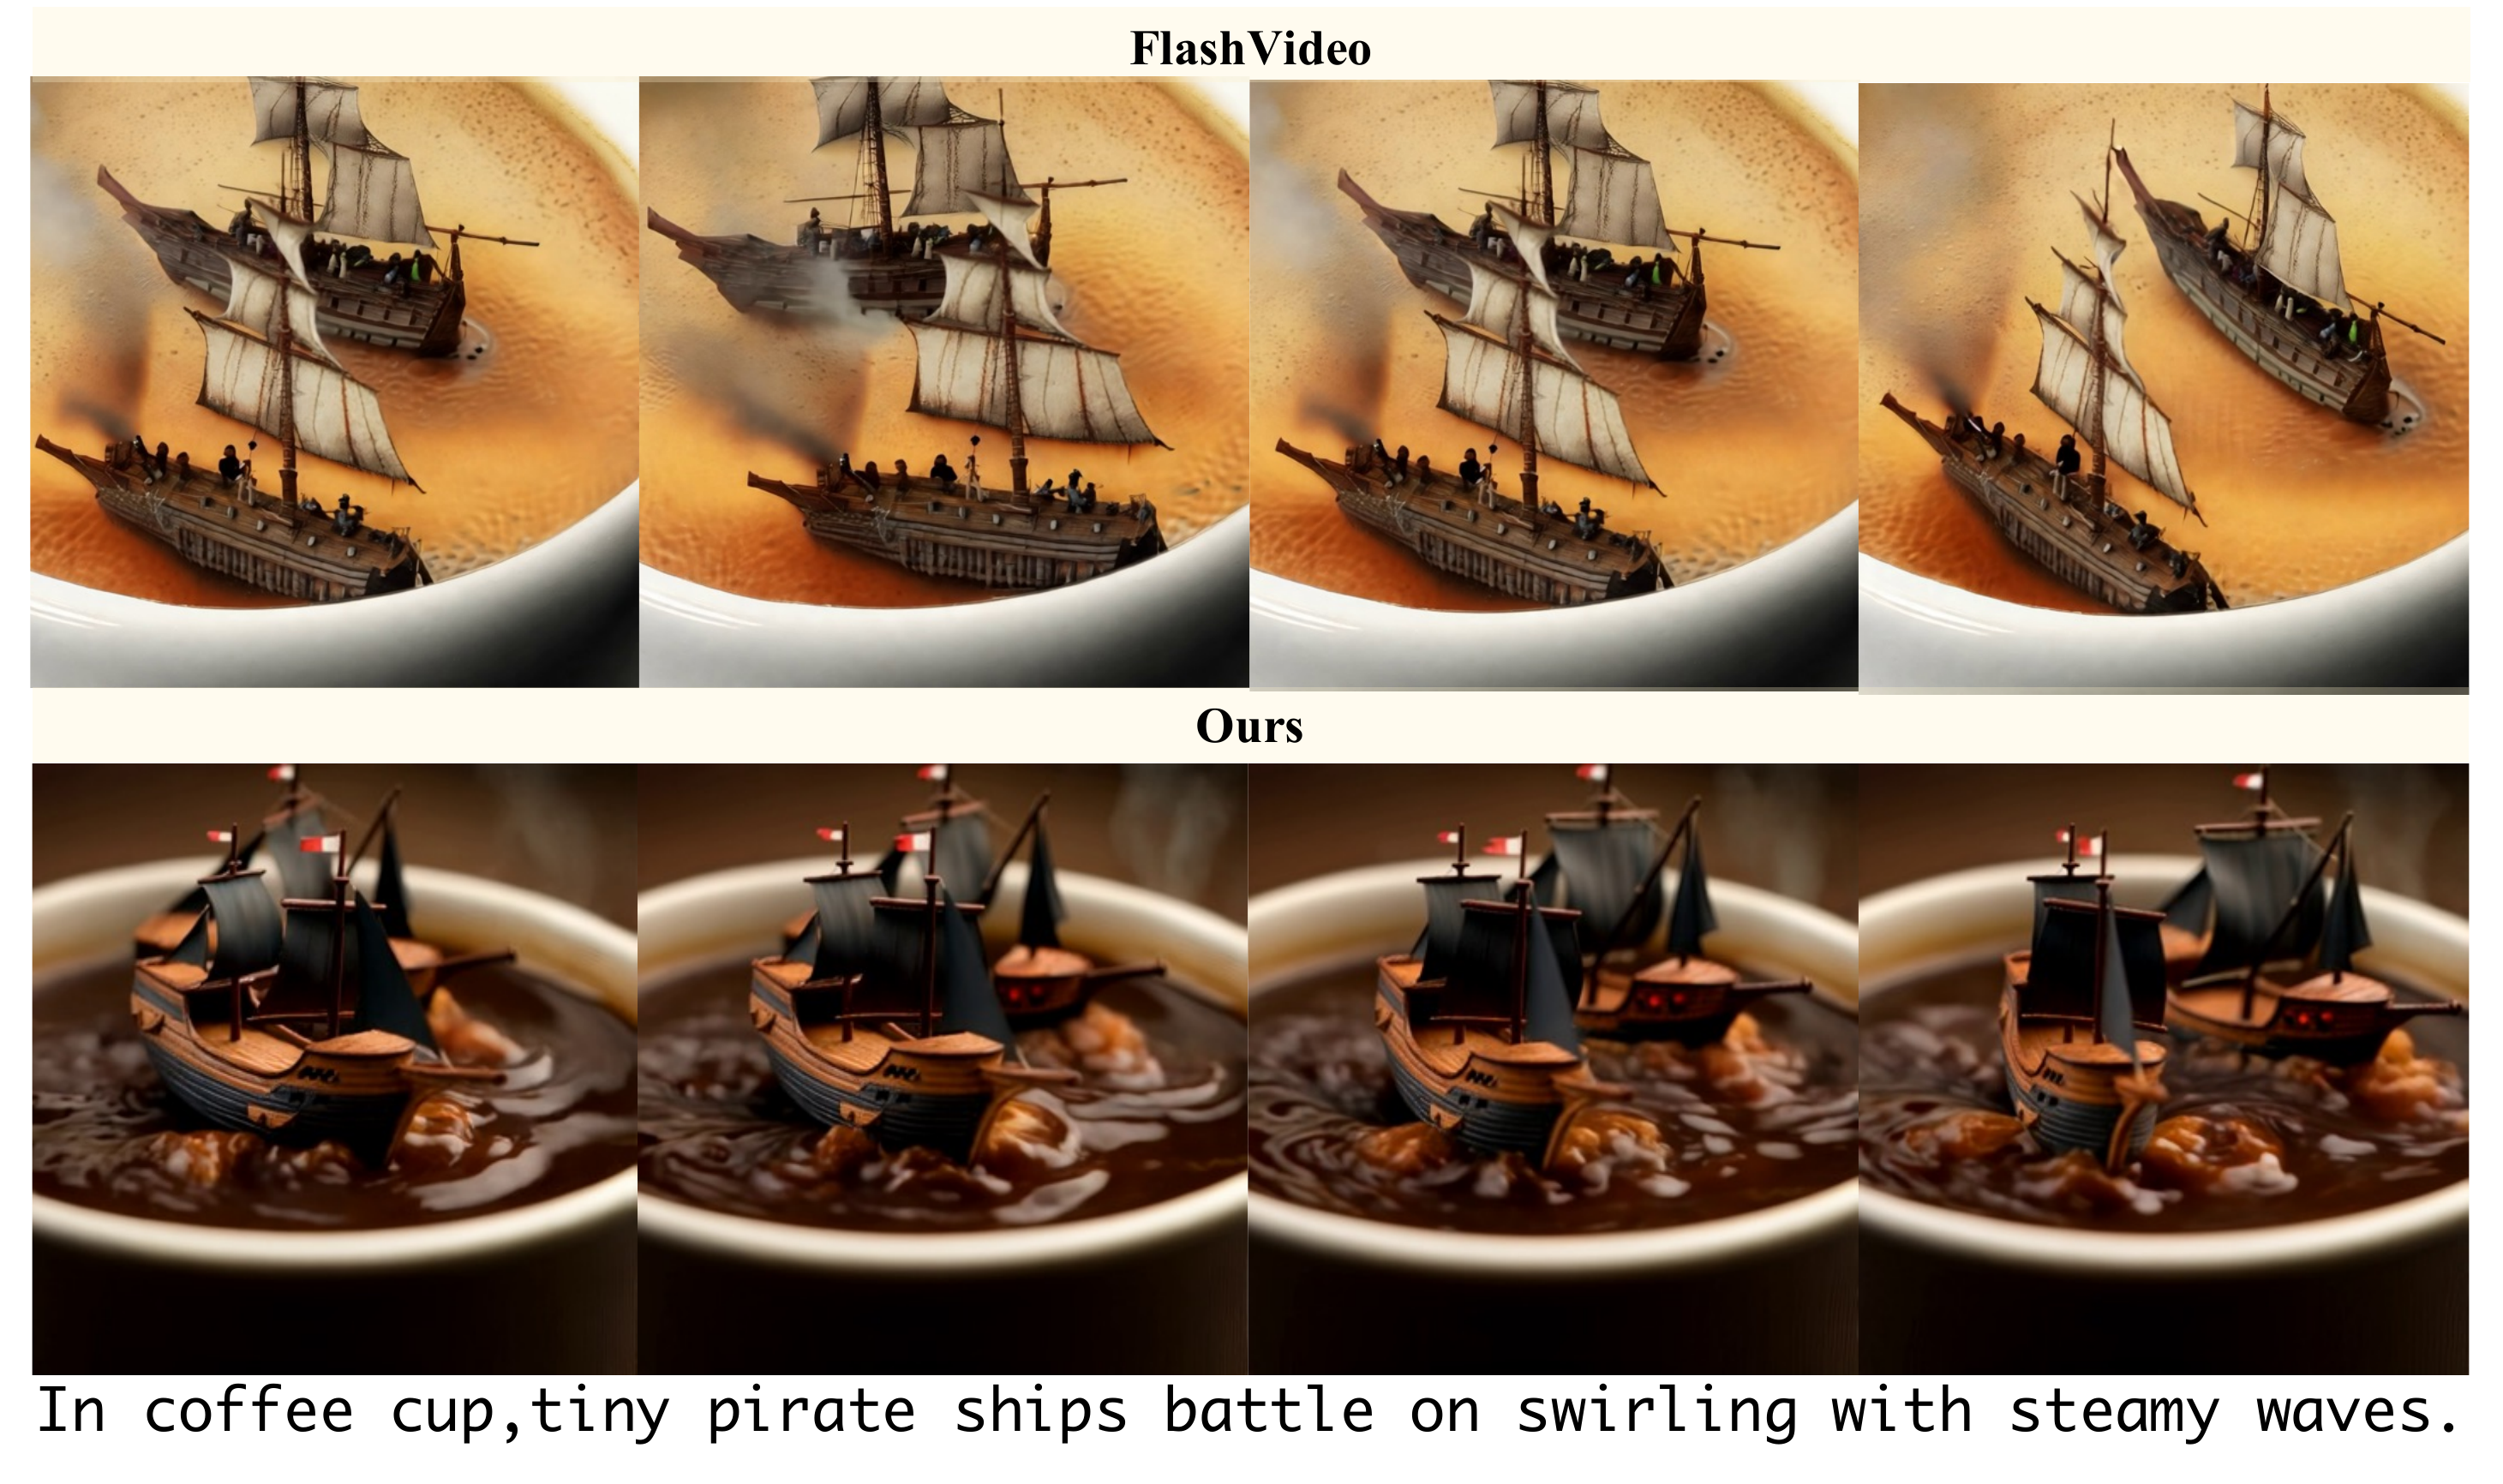} 
\vspace{-10pt}
\caption{%
    \textbf{Visual Comparisons between \method and FlashVideo.}  
    Our results exhibit a notably more imaginative and aesthetically pleasing scene of pirate ships in a coffee cup, compared to FlashVideo. The texture in our results is rendered with greater delicacy, vividly capturing the "steamy waves."
}
\label{fig:CompareVSRflashvideo}
\end{figure}

As for the Refine stage, we provide more visual results.  
As shown in Fig.~\ref{fig:CompareVSRframe}, our method demonstrates significant success in rendering details such as the cat's paw and the drone's shape.  
We also present a sequence of four frames in Fig.~\ref{fig:CompareVSRvideo} to further compare VEnhancer with our method.  
While both methods generate clear videos, \method handles dynamic details more effectively.

\begin{figure}[t]
\centering 
\includegraphics[width=0.98\linewidth]{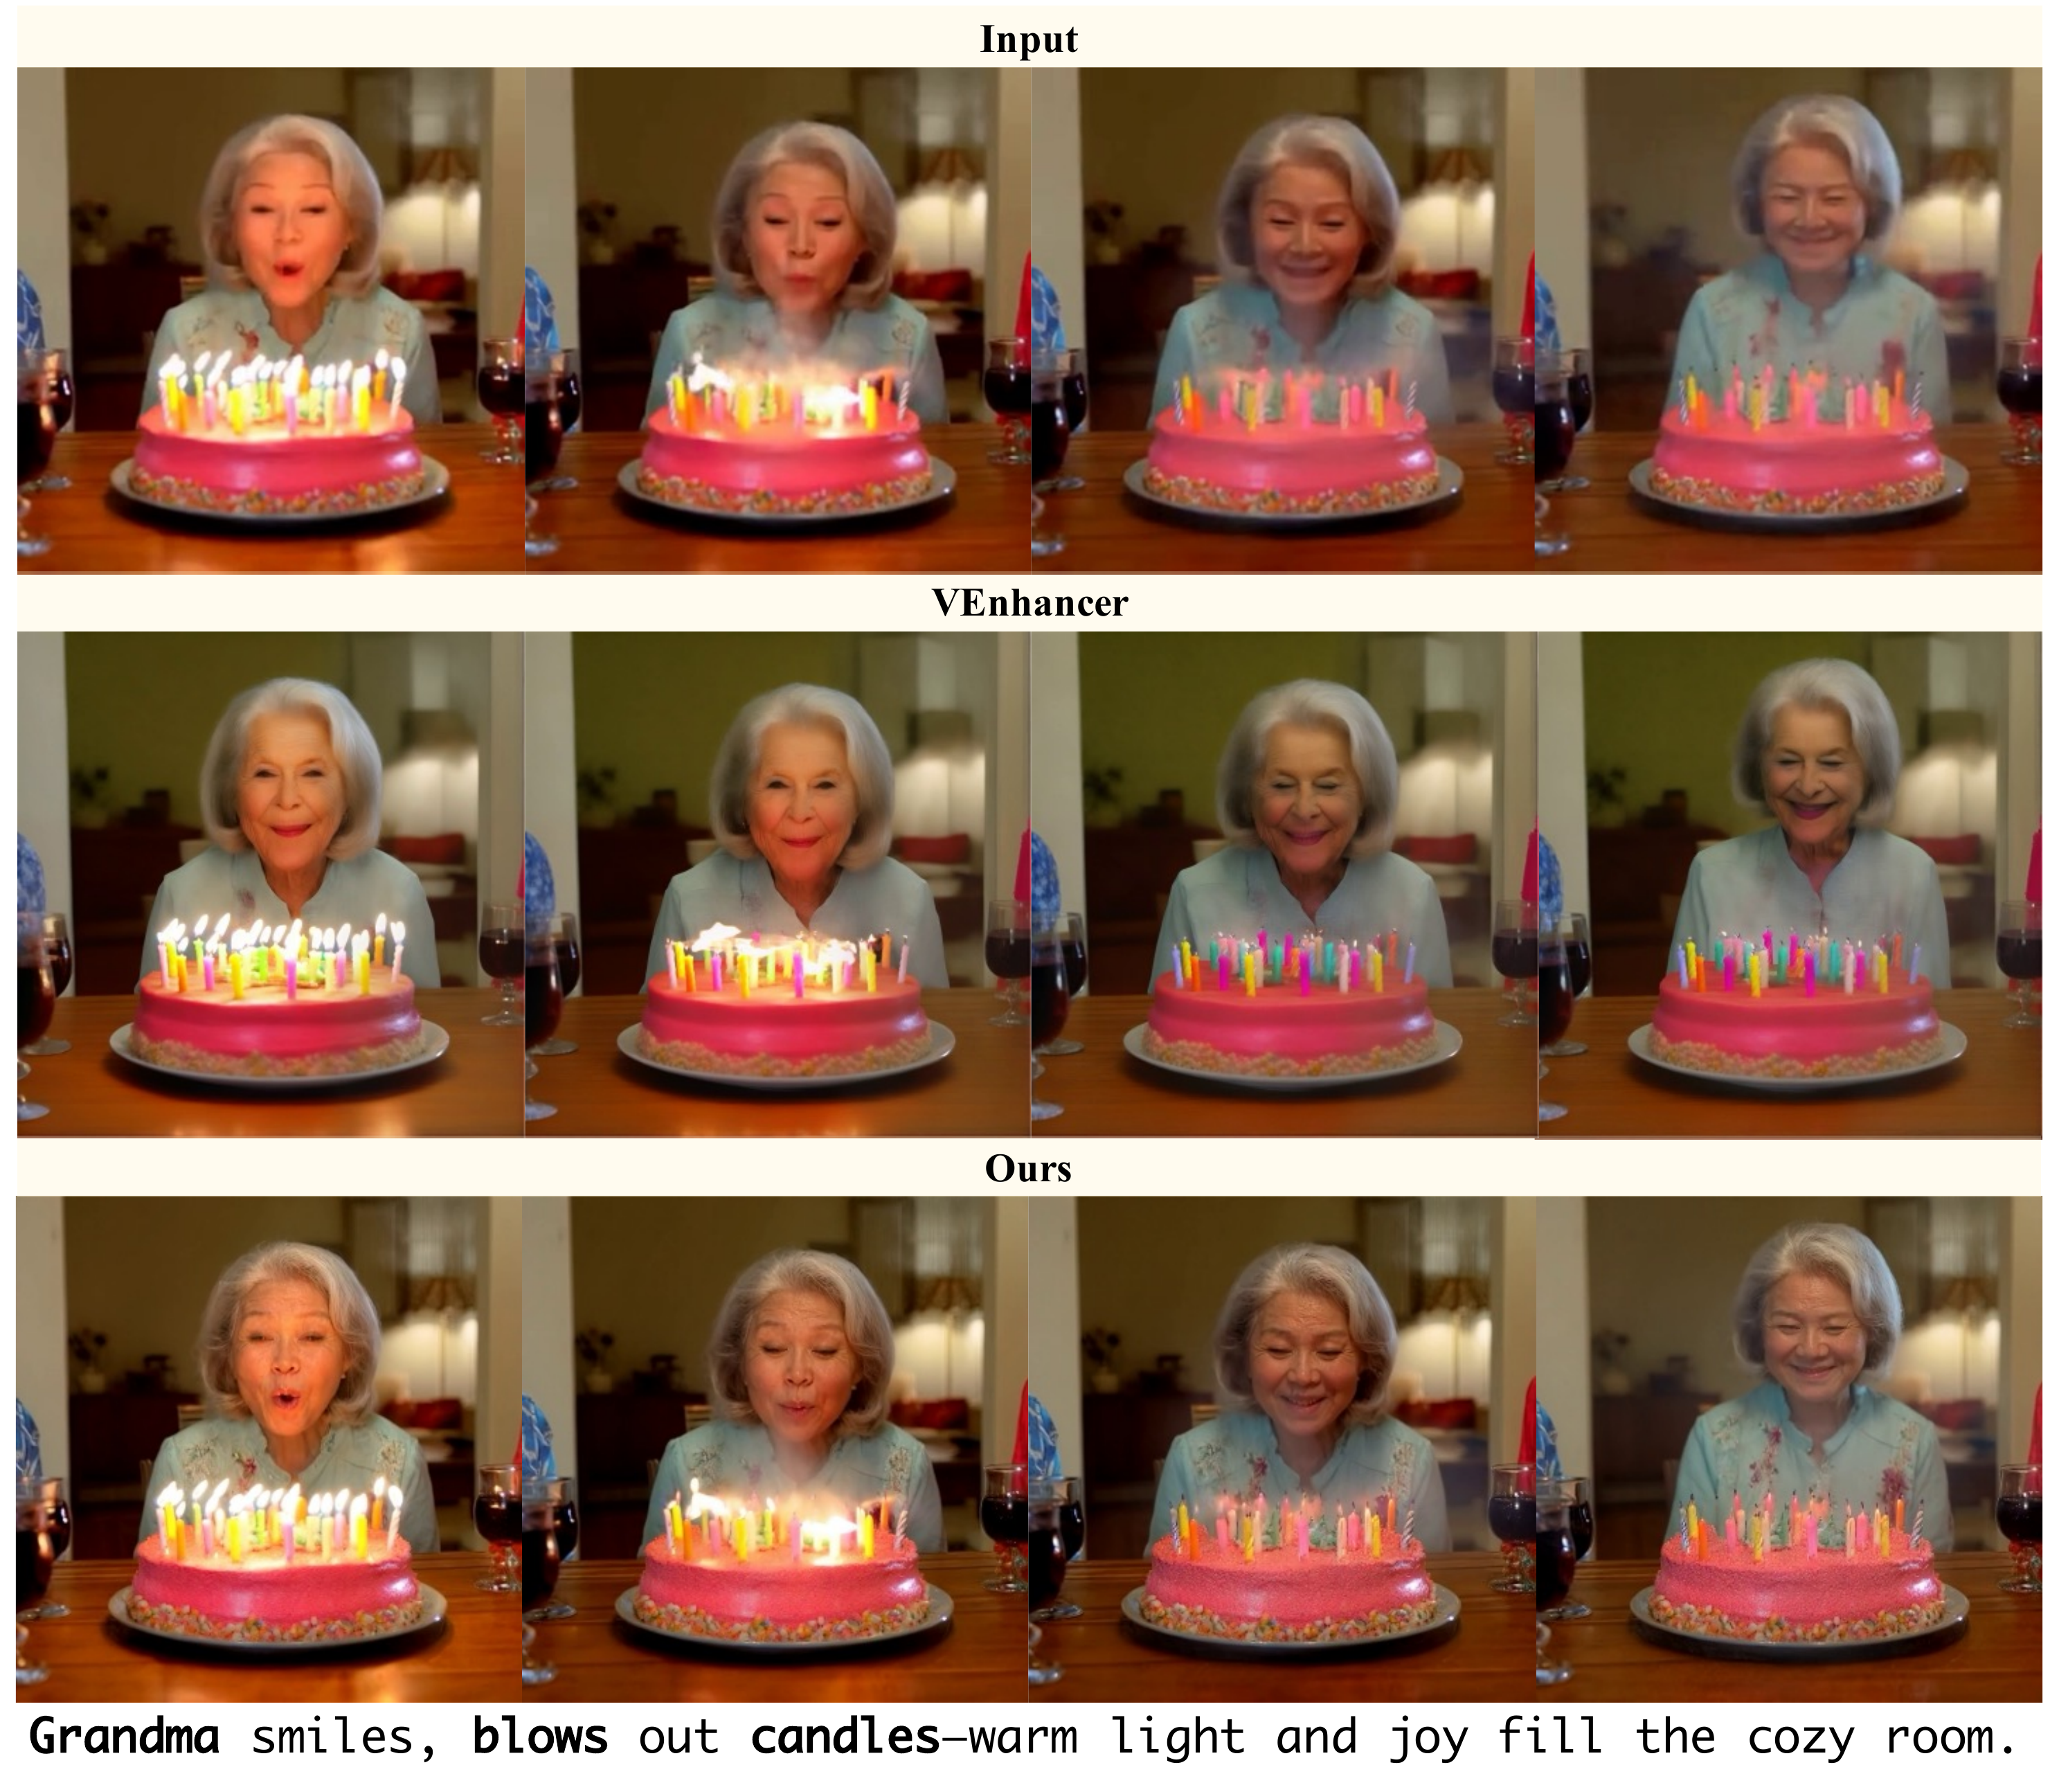} 
\vspace{-10pt}
\caption{%
    \textbf{Comparison of fine-grained facial expressions and intricate details.}  
    Example from a video clip with significant changes in a grandmother's facial expressions. VEnhancer struggles with facial identity, inaccurate lip articulation, and ambiguous candle flickering. In contrast, \method (Ours) intelligently refines these details, realistically augmenting them while maintaining consistency.
}
\label{fig:CompareVSRvideo}
\end{figure}

\subsection{Ablation Studies}

\paragraph{Shift window attention.}
We provide quantitative results in Tab.~\ref{tab:ablatesw} to further analyze the effect of shift-window attention on video generation.  
Our method achieves a shorter runtime while preserving finer details, demonstrating that when handling high-resolution video, we can focus on a local receptive field to refine details.

\begin{table}[t]
\centering
\small
\caption{\textbf{Ablation study}. Highest value in \textbf{bold}.}
\setlength{\tabcolsep}{3pt}
\begin{tabular}{lcccccc}
\toprule
\textbf{Method} & \textbf{QS $\uparrow$} & \textbf{AQ $\uparrow$} & \textbf{DD $\uparrow$} & \textbf{MS $\uparrow$} & \textbf{OC $\uparrow$} & \textbf{Time$\downarrow$}\\
\midrule
\method w/o SW & 82.94 & 66.82 & 69.44 & \textbf{98.12} & \textbf{27.41} & 107s \\
\method & \textbf{83.24} & \textbf{66.86} & \textbf{72.22} & 97.95 & 27.38 & \textbf{76s} \\
\bottomrule
\end{tabular}
\label{tab:ablatesw}
\end{table}

\begin{figure}[t]
    \centering
    \includegraphics[width=0.48\textwidth]{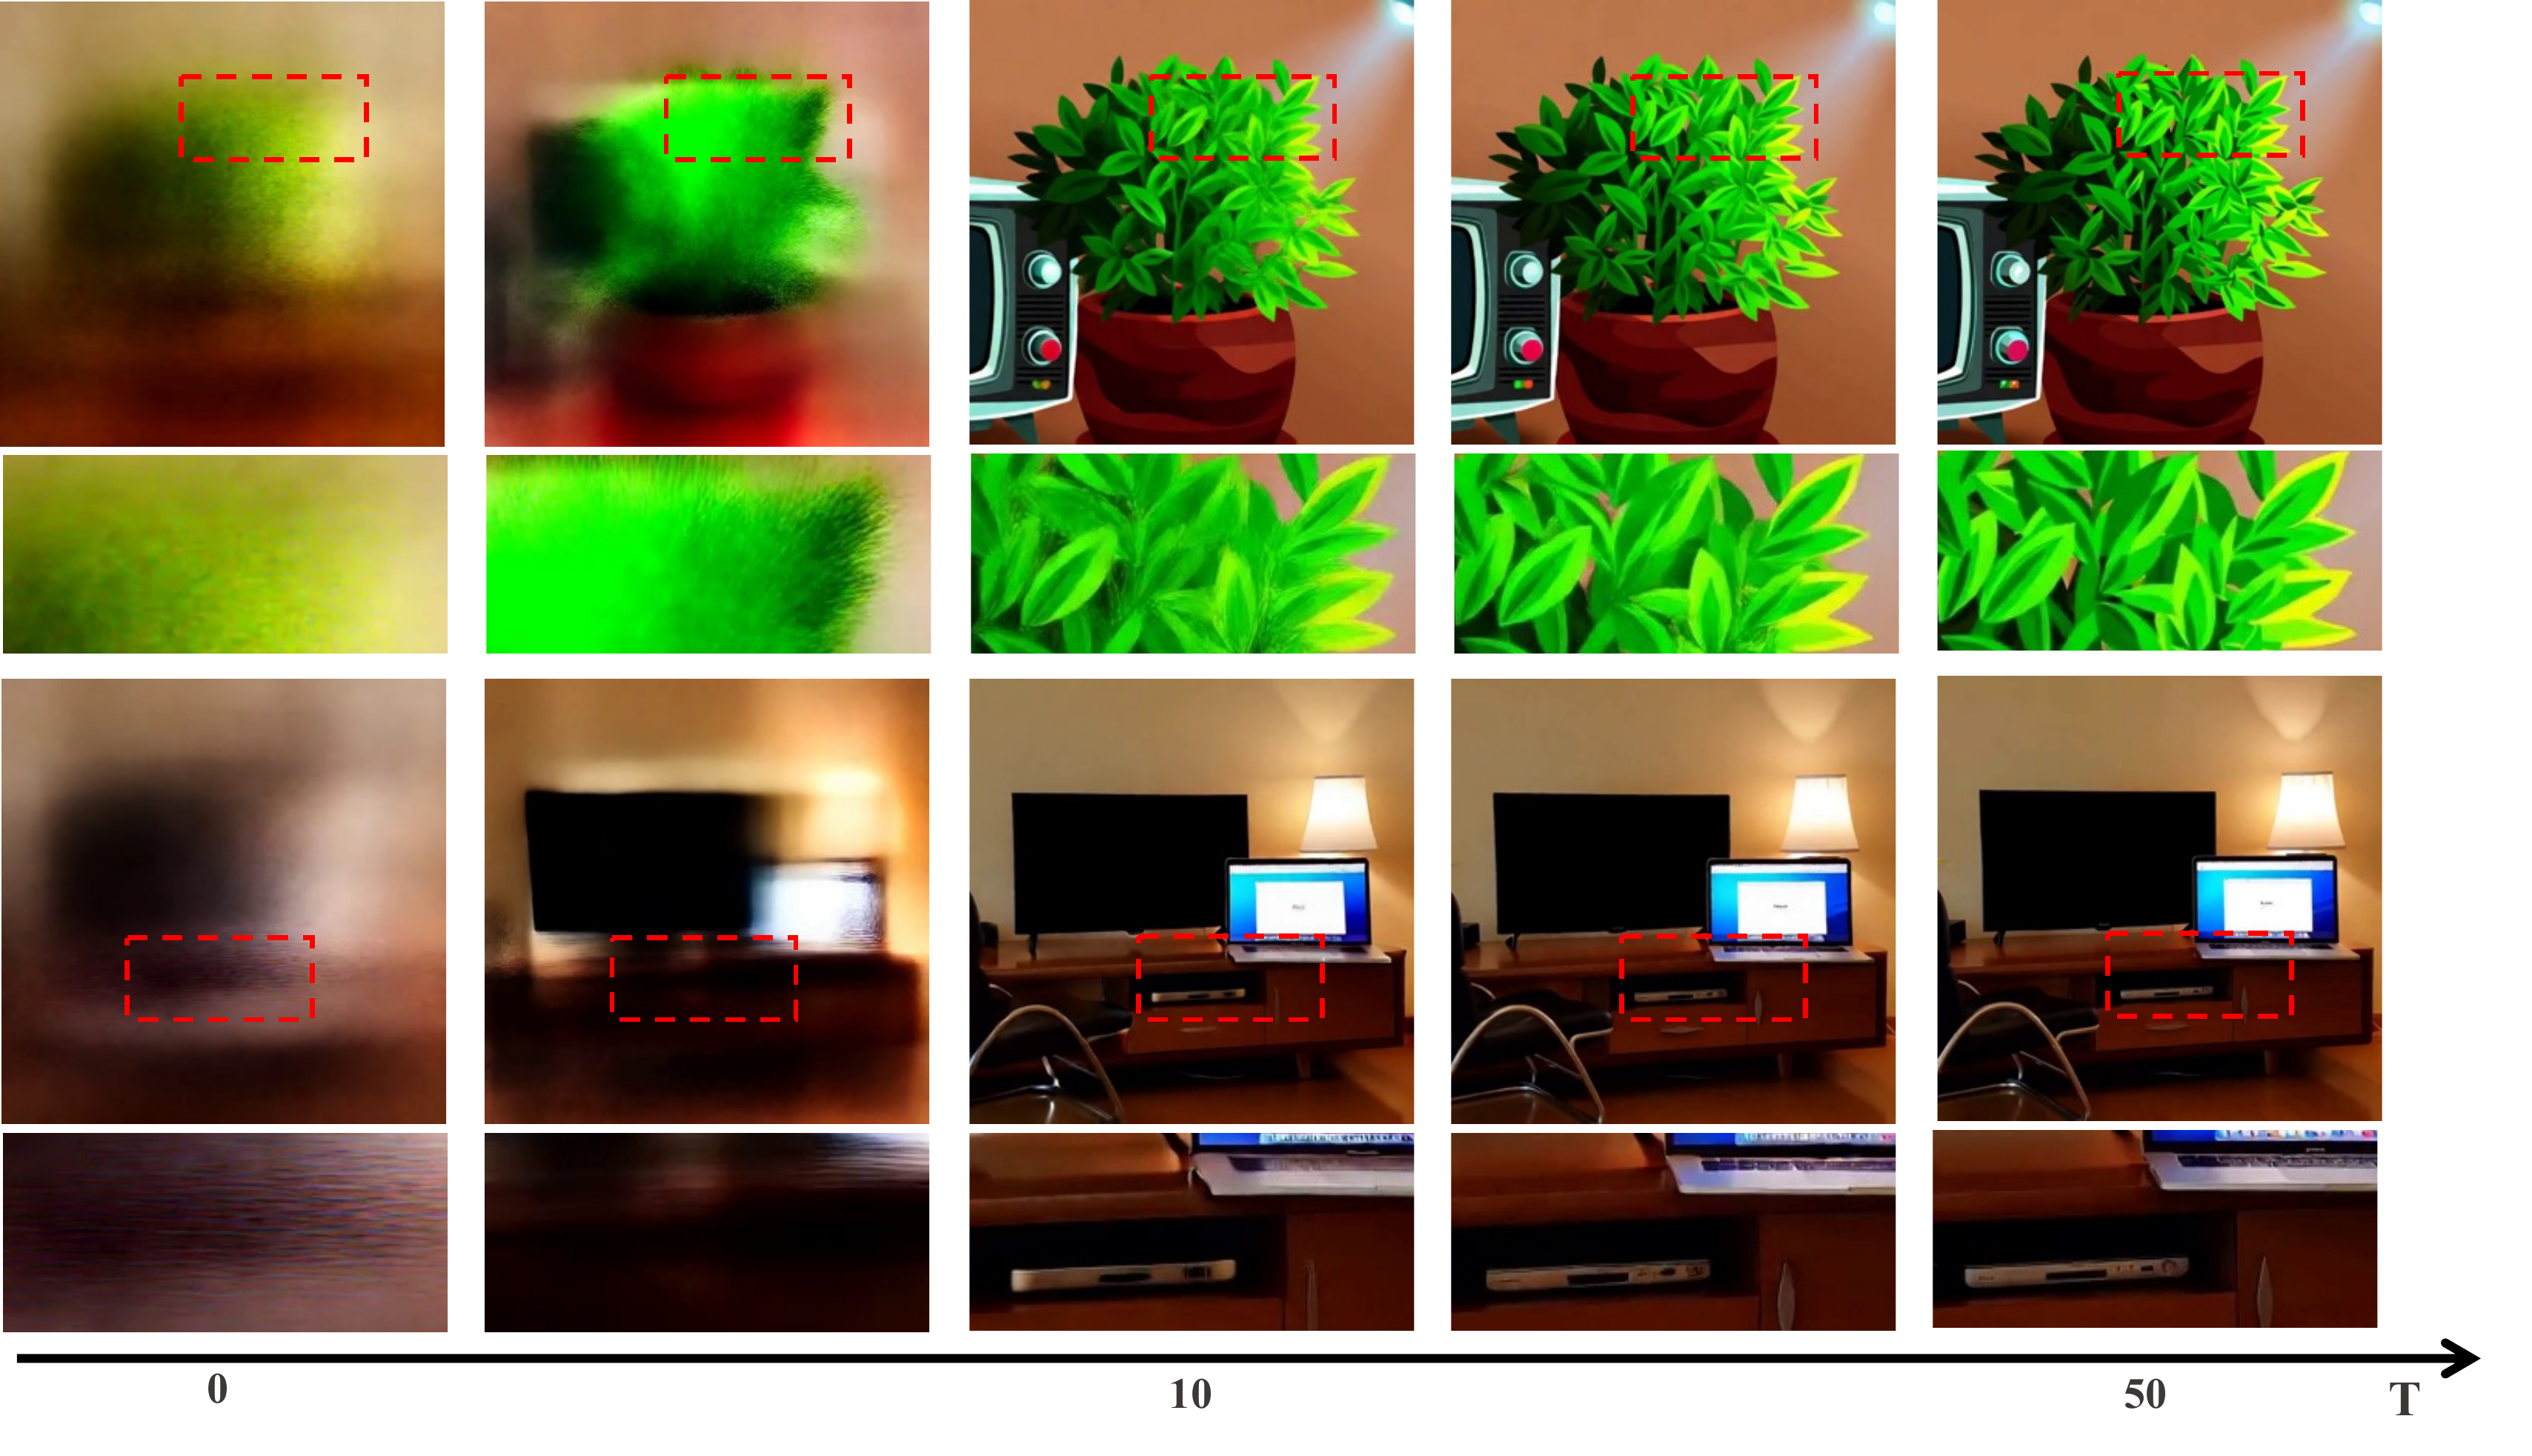}
    \caption{
        \textbf{Visualization of the denoising process.}
        The overall structure emerges rapidly within the first few denoising steps (around 10), with subsequent steps focusing on refining fine-grained details.
    }
    \label{fig:frequency-divided}
\end{figure}
\paragraph{Step division.}
Furthermore, we visualize the changes in video content during the denoising process, as shown in Fig.~\ref{fig:frequency-divided}.  
We observe that the overall structure emerges rapidly within the first few denoising steps (around 10), with the remaining steps dedicated to progressively refining fine-grained details.  
Thus, we choose the denoising step to be around 10 and visualize the results of the refiner under different inference hyperparameters in Fig.~\ref{fig:ablation_changestep}. 

\begin{figure}[t]
    \centering 
    \includegraphics[width=0.98\linewidth]{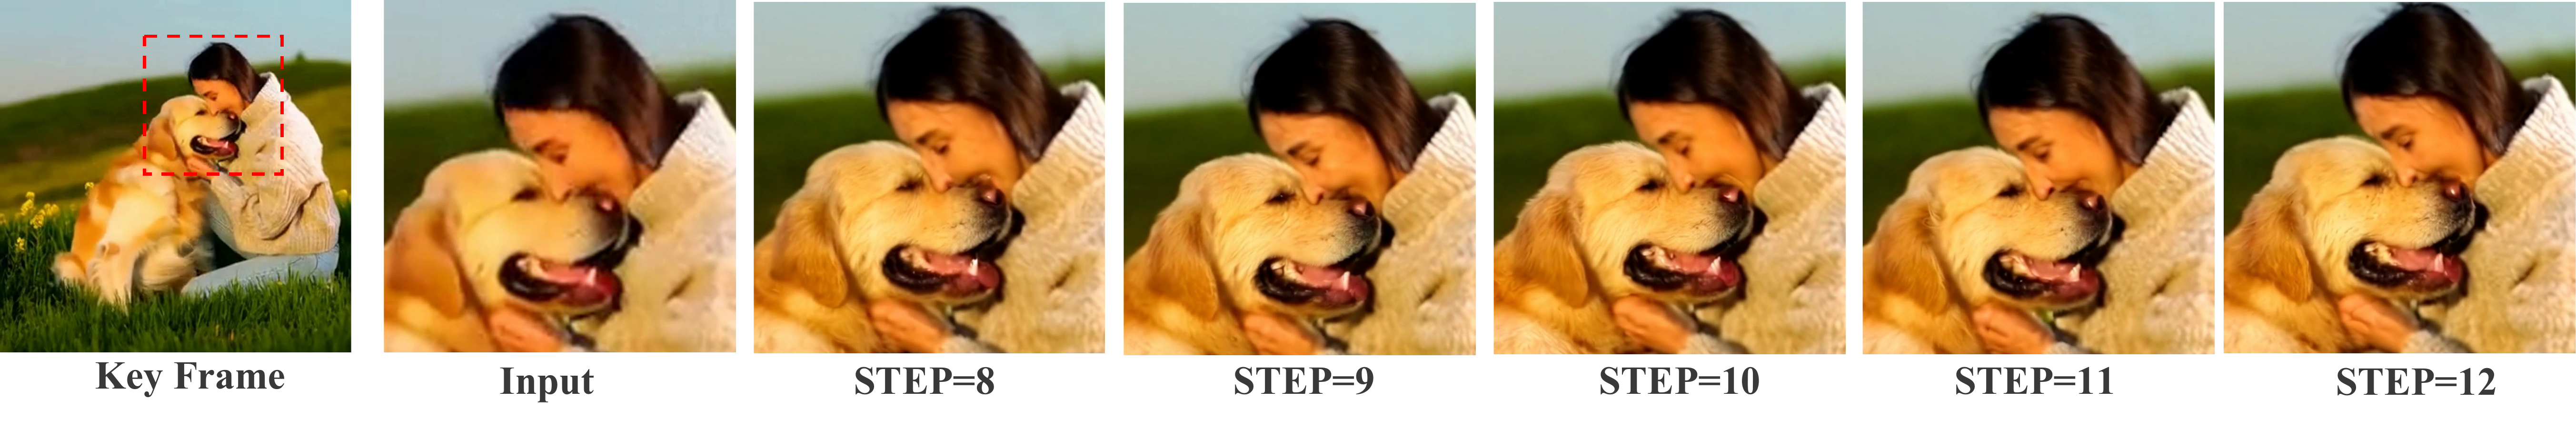} 
    \vspace{-10pt}
    \caption{%
            \textbf{Results of the refiner under different inference hyperparameters.}
    }
    \label{fig:ablation_changestep}
    \vspace{-10pt}
\end{figure}

\section{Teaser Prompt List}
We provide our prompt list for the generated videos presented in Teaser. %
\begin{promptbox}
1. A charming panda, dressed in a chef's hat and red apron, chops vegetables in a rustic kitchen. It stirs a pot, tastes the soup, and plates a beautifully arranged dish, exuding delight.
    
2. A girl spins in the starry night sky, her shimmering pastel costume and floating feathers captured in a dreamy anime illustration.
    
3.A playful corgi with golden fur trots along a tropical beach, wearing blue sunglasses. The camera follows it as it walks along the shoreline, pauses, and enjoys the sun and waves.
\end{promptbox}

\section{Limitations and Future Work}
Although our method is theoretically capable of generating videos at arbitrarily high resolutions, in practice it is constrained by computational resources.
Specifically, our experiments show that the current implementation can stably support resolutions up to $2048 \times 2048$, while higher resolutions will lead to out-of-memory (OOM) errors on A800(80G).
As part of future work, we plan to integrate patch-based spatial division strategies or memory-efficient attention mechanisms to further extend the scalability of our approach, enabling efficient training and inference at ultra-high resolutions.
%
% \section{LLM Usage}
% \label{appendix:llm_usage}
% We used a large language model (LLM) \emph{only for writing polish}, including grammar correction, phrasing refinement, and improvements to clarity and readability.
% The LLM did \emph{not} contribute to research ideation, problem formulation, method design, experimental setup, result selection, interpretation, or drafting of technical content (theorems, algorithms, proofs, metrics, or analyses).
% All technical claims, experiments, figures, tables, and conclusions were conceived, implemented, and verified by the authors.

\section{More quality results}\label{supp:quality_results}
We have provided additional comparison cases, as shown in Fig.\ref{supp:1} and Fig.\ref{supp:2}.

\begin{figure*}[t]
    \centering 
    \includegraphics[height=\textheight]{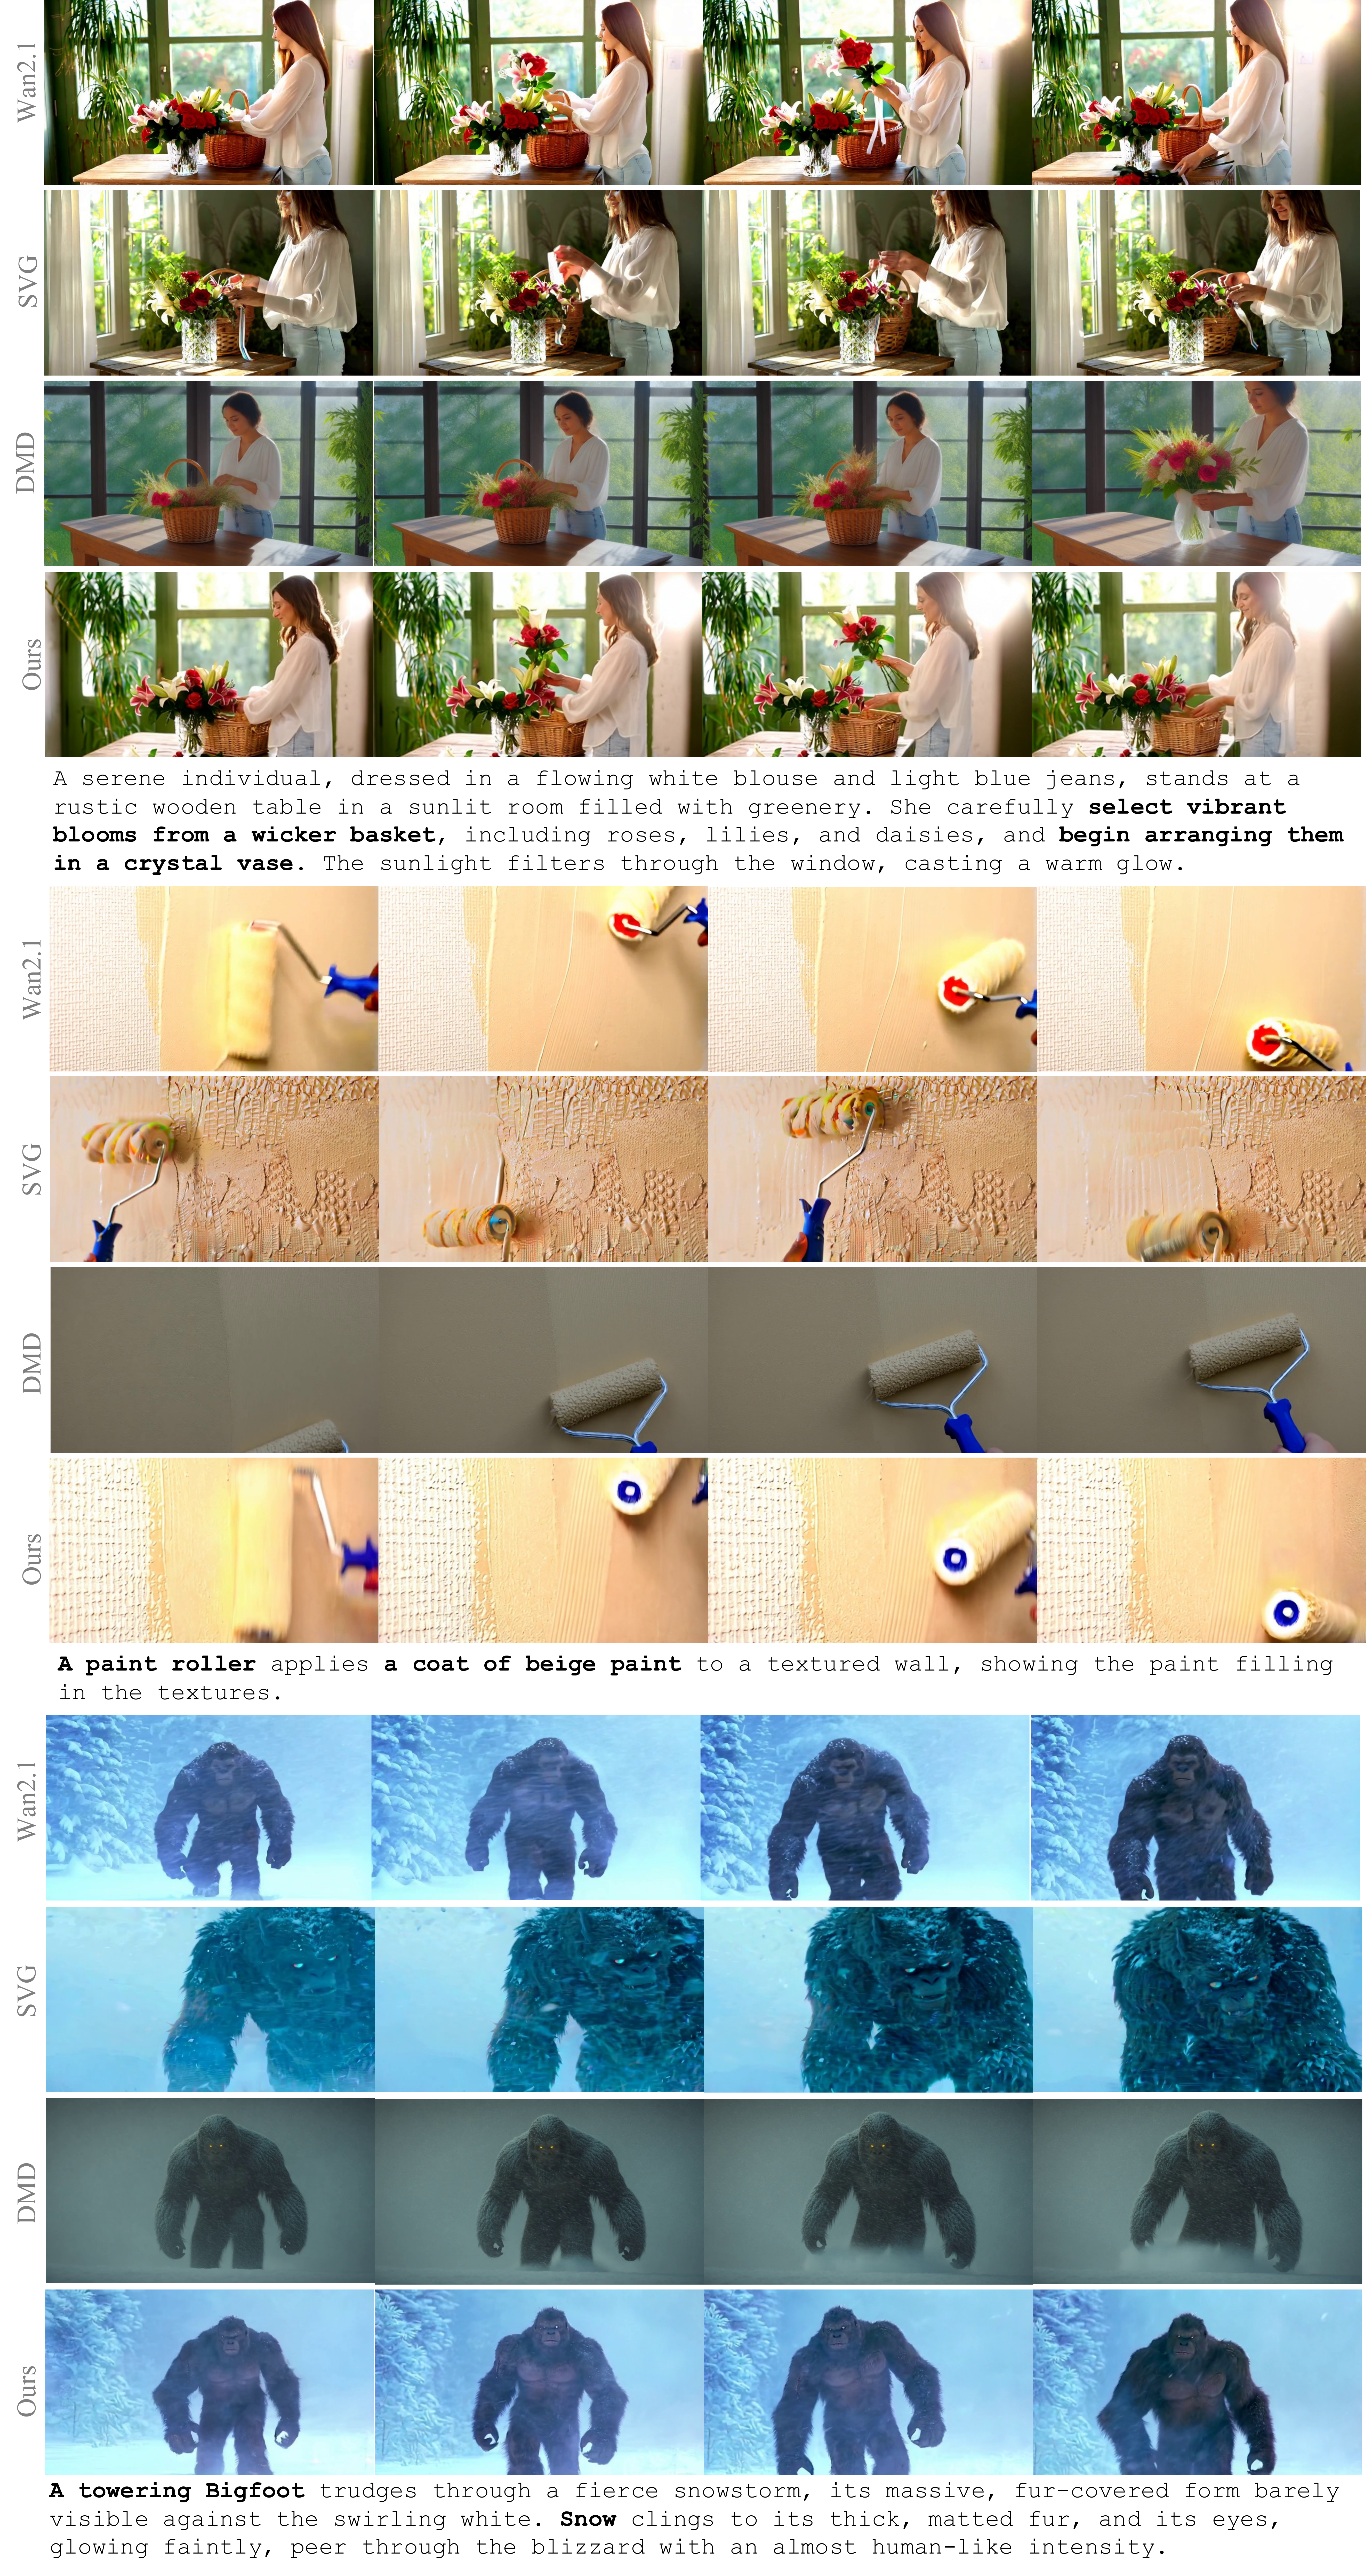} 
    \caption{%
            \textbf{Comparisons.} From top to bottom, each four videos is from the same setting.
    }
    \label{supp:1}
    \vspace{-10pt}
\end{figure*}
\begin{figure*}[t]
    \centering 
    \includegraphics[height=\textheight]{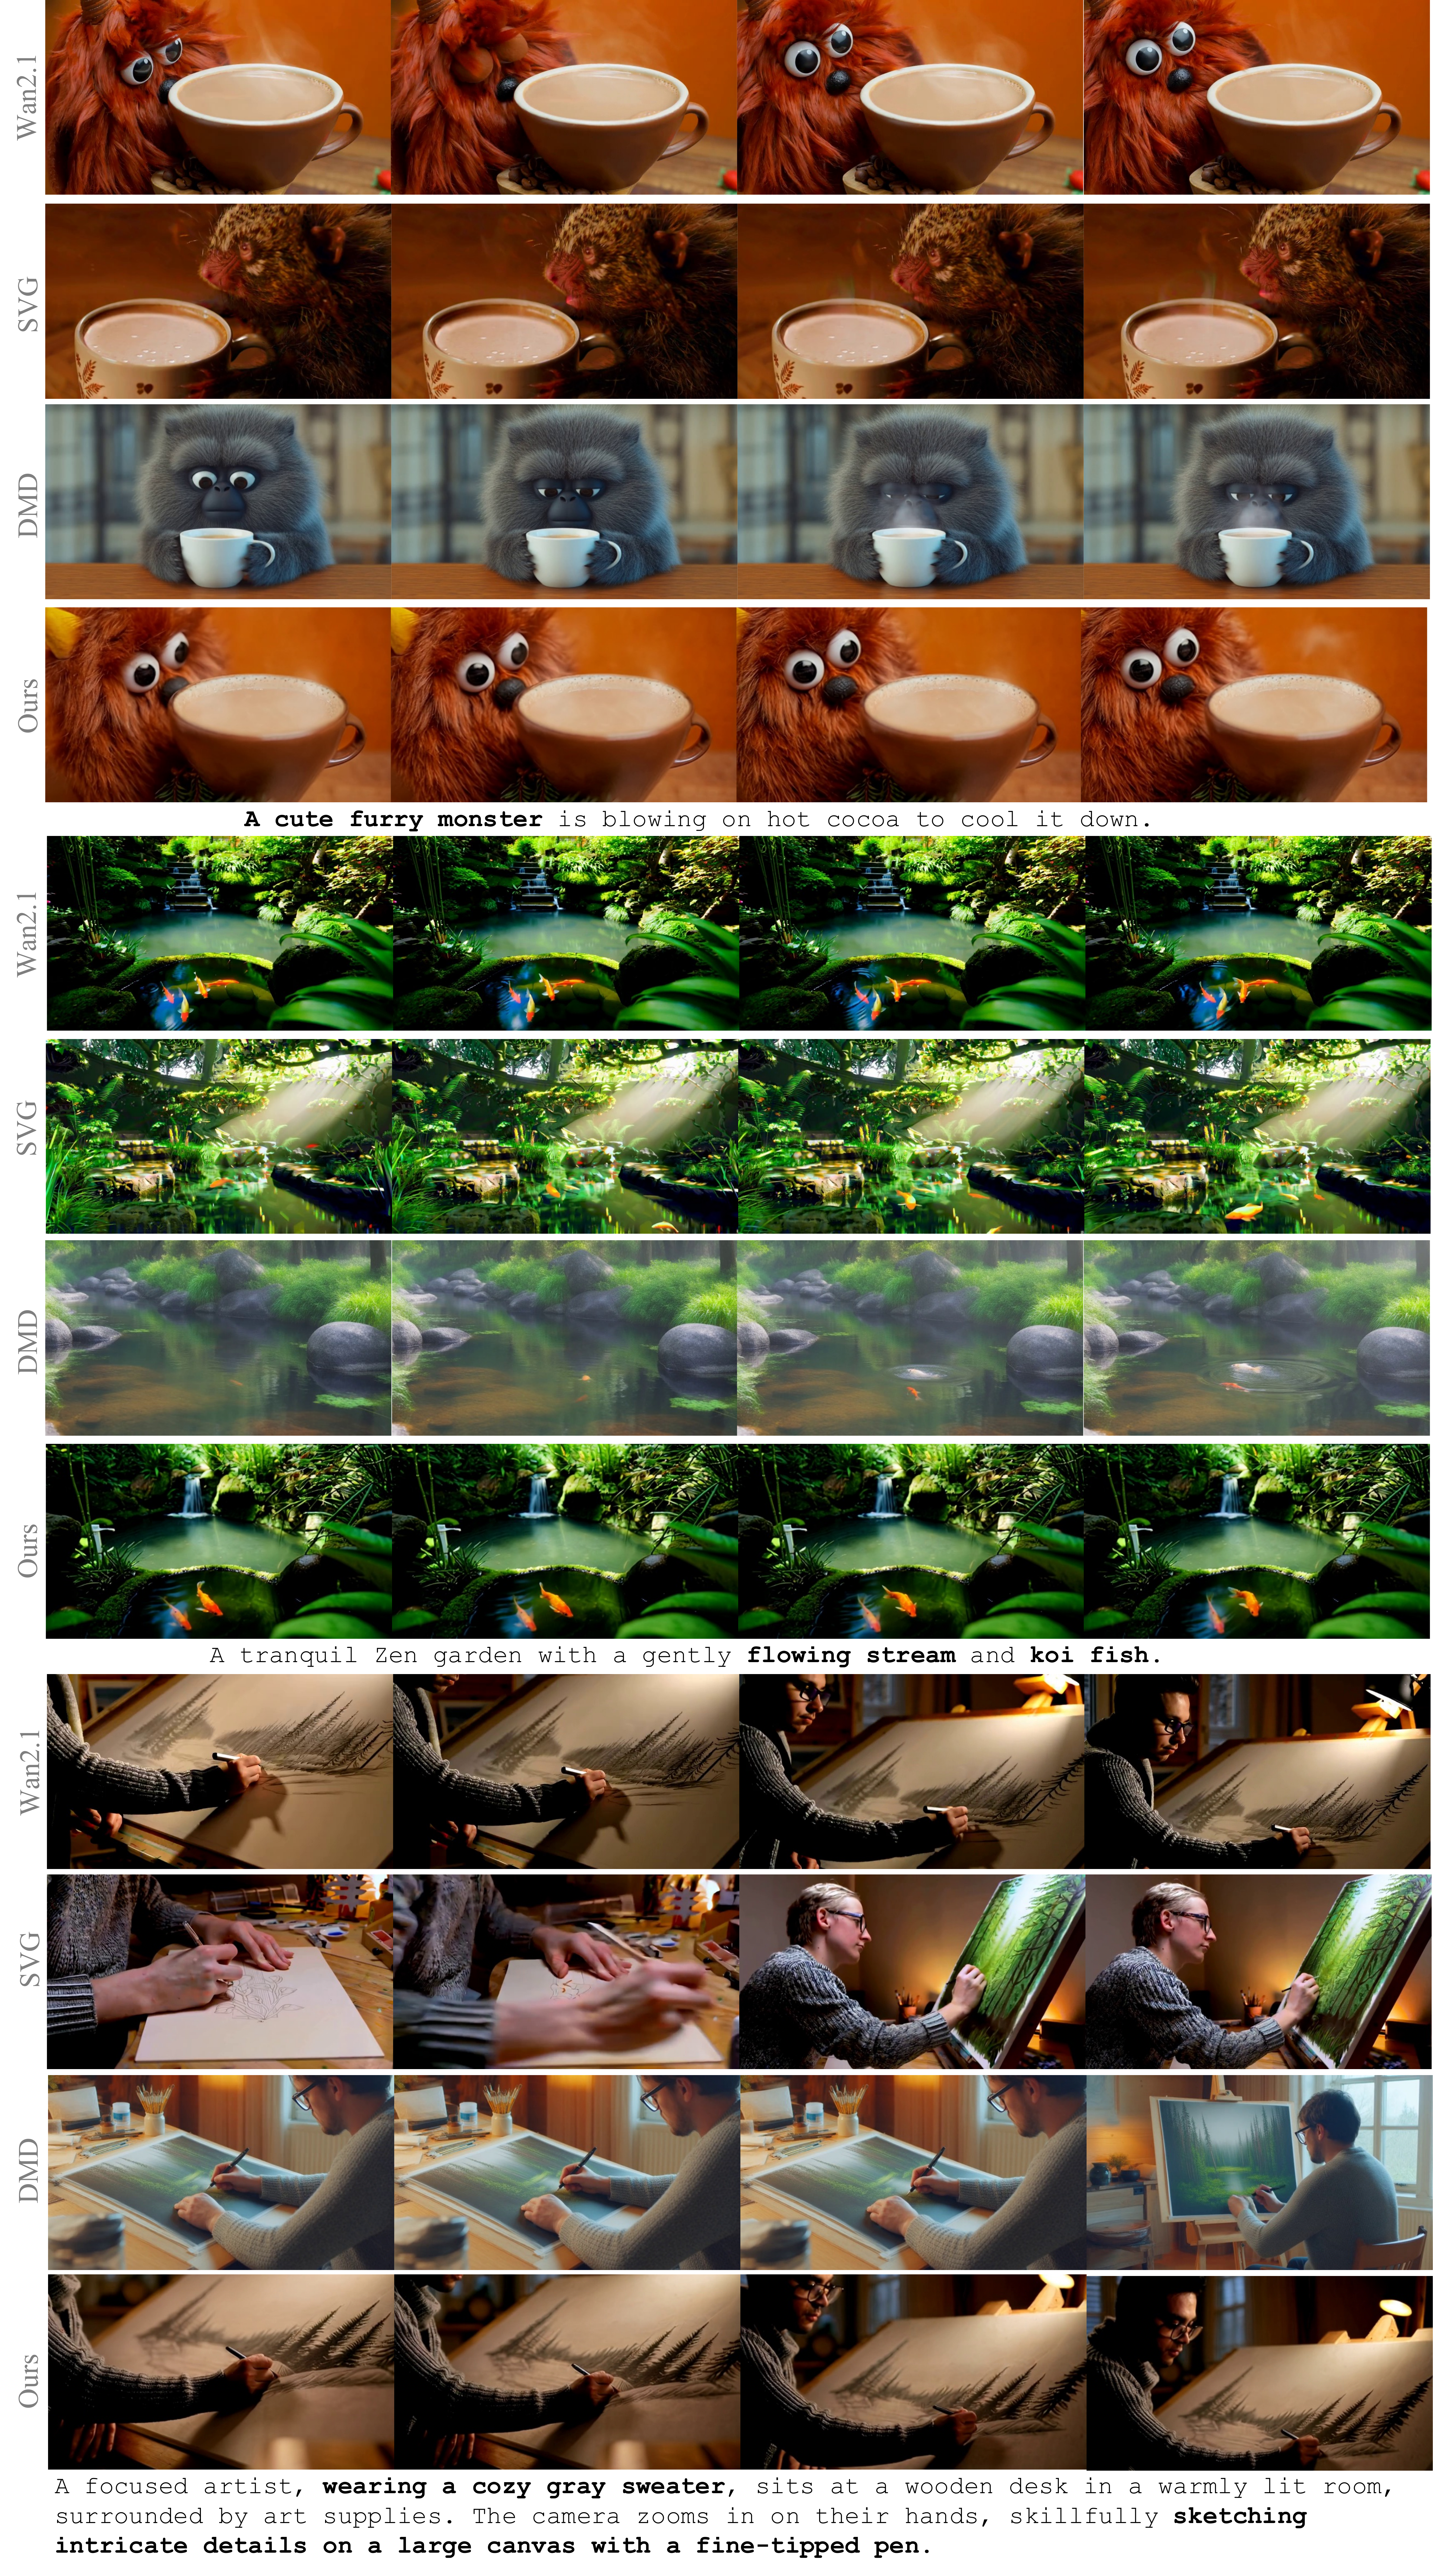} 
    \caption{%
            \textbf{Comparisons.} From top to bottom, each four videos is from the same setting.
    }
    \label{supp:2}
    \vspace{-10pt}
\end{figure*}
